# Supplementary material for: Time-scale effects on the gain-loss asymmetry in stock indices
Source: arXiv:1608.04506 ancillary file (2016-08-17)
Supplement: Supplementary file 1 [file suppl_mat.pdf]

# Supplementary Material for "Time-scale effects on the gain-loss asymmetry in stock indices"

Bulcsú Sándor,[1,2] Ingve Simonsen,[3] Bálint Zsolt Nagy,[4] and Zoltán Néda[2,*]

[1] *Goethe University Frankfurt, Institute for Theoretical Physics, D-60438, Frankfurt am Main, Germany*

[2] *Babeş-Bolyai University, Department of Physics, RO-400084, Cluj-Napoca, Romania*

[3] *Norwegian University of Science and Technology, Department of Physics, NO-7491 Trondheim, Norway*

[4] *Babeş-Bolyai University, Department of Economics, RO-400084, Cluj-Napoca, Romania*

(Dated: July 13, 2016)

* zneda@phys.ubbcluj.ro

## THE SHUFFLED TIME-WINDOW METHOD

As discussed in Sec. IV of the paper, the shuffled time-window method applied to the time-series of the S&P500 and NASDAQ100 indices, leads to the similar results to the ones reported for the DJIA index. Here we present, analogously to figures of the paper, the variation of the inverse statistics after shuffling the $r_1(t)$ daily returns. As expected, complete shuffling, i. e. using time window $T = 1$, leads to symmetric investment horizon distributions (compare the top panels of Fig. 1 and Fig. 2 for the S&P500 and NASDAQ100 indices, respectively). On the other hand, a time window $T = 25$ reproduces the asymmetry found in the original indices (see the bottom panels of Fig. 1 and Fig. 2).

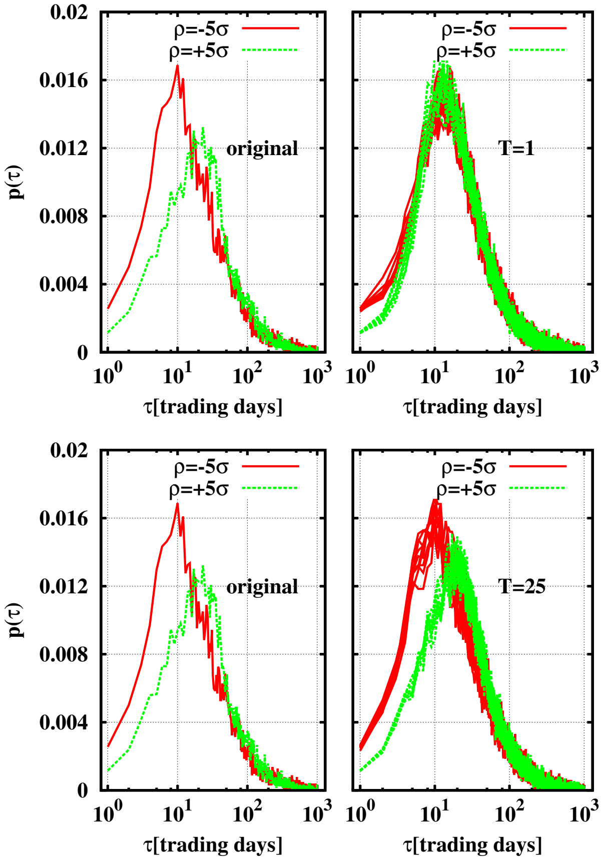


FIG. 1. Left: The investment horizons distributions of the original SNP500 index. Right: The inverse statistics for the shuffled version of the index using time windows of $T = 1$ and $T = 25$ trading days in the top and bottom panels respectively. The superimposed curves with the same colour correspond to different permutations. The return levels considered for the inverse statistics are five times larger than the volatility of returns: $|\rho| = 5\sigma \approx 5\%$.

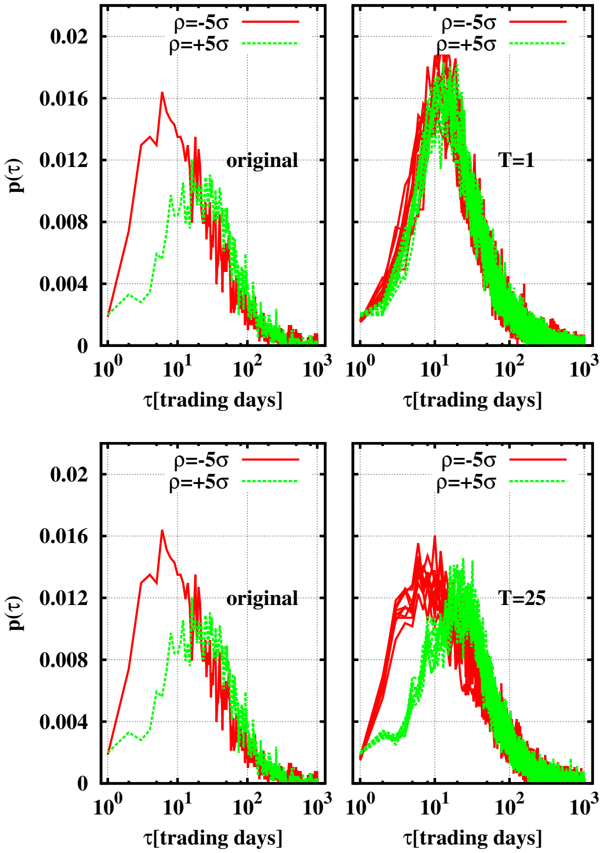


FIG. 2. Left: The investment horizons distributions of the original NASDAQ100 index. Right: The inverse statistics for the shuffled version of the index using time windows of $T = 1$ and $T = 25$ trading days in the top and bottom panels respectively. The superimposed curves with the same colour correspond to different permutations. The return levels considered for the inverse statistics are five times larger than the volatility of returns: $|\rho| = 5\sigma \approx 5\%$.
